# Supplementary material for: Incentivizing Truthfulness Through Audits in Strategic Classification
Source: arXiv:2012.09147 source file (2020-12-16)
Supplement: Supplementary file 1 [file supplement.tex]

\section*{Supplementary Materials}

\subsection*{Proof of Proposition~\ref{thm:impossibility}}

%\begin{proof} 
    %As stated previously, 
    When resources are allocated via threshold, this result is straightforward.
    In the case of top-$k$, the need for auditing can be seen by a simple two agent example for any arbitrary score function.
    Let $n = 2$ and $k = 1$. 
    Given $f:\inter \rightarrow \R$, assume by way of contradiction that $f$ induces truthful reporting to be an equilibrium, but has $f(\x, \z) \neq f(\x)$.
    Then there exists some values $\x\in I^{d}, \z_1, \z_2 \in I^{s}$ with $f(\x, \z_1) \neq f(\x, \z_2)$. WLoG assume $f(\x, \z_1) > f(\x, \z_2)$. Let $\aj_1 = (\x, \z_1)$ and $\aj_2 = (\x, \z_2)$. 
    Since $k= 1$, agent $2$ will never receive the resource unless they report $\z_2' = \z_1 \neq \z_2$.
    Therefore reporting truthful $\z$ can be an equilibrium iff $\forall (\x, \z) \in \inter$, $f(\x, \z) = f(\x)$.
%\end{proof}

\subsection*{Proof of Theorem~\ref{thm:thresh_audit_hard}}
    To show the hardness of optimally auditing we will reduce from SAT. Before showing this reduction, we make the following observation about optimal auditing.
    Suppose an agent reports type $\aj_i' = (\x_i, \z_i')$, by definition the principal is sure that $\x_i$ is reported truthfully, but may be sure about the veracity of $\z_i'$. 
    However, in some cases the principal may know for certain if $\z_i'$ was reported truthfully. One such case, which we will make use of, is when for all $\z\in I^s$ with $\z\neq \z_i'$, we have $h(\x_i, \z) = 0$. 
    
    For a given Boolean $\Phi$, over variables $b_1, \dots b_m$, we will encode $\Phi$ into the distribution over agent types, given by $D$, such that it is NP-hard to determine if for some reported $(\x_i, \z_i')$ there exists another $(\x_i, \z)$ with $\z \neq \z_i$ and $h(\x_i, \z)> 0$.
    Suppose that $I = \{0, 1\}$, i.e. agent features are binary, set $d = 2$, and $s = m$, the agents are of the form $\langle x_1, x_2, z_1, \dots z_m\rangle$. 
    Define the PDF of $D$ over $I^2\times I^s$ as 
    \begin{align*}
        h(\x, \z) = 
                \begin{cases}
                    \frac{1}{2^{m + 1}} & \text{ if } x_1 = 1, x_2 = 1, \text{ and } \z = 1\\ 
                    \frac{1}{2^{m +1}} &\text{ if } x_1 = 1, \z \neq 1, \text{ and } x_2 = \Phi(\z)\\
                    \frac{1}{2^{m + 1}} & \text{ if } x_1 = 0\\
                    0 &\text{ otherwise}
                \end{cases}
    \end{align*}
    Lastly, suppose that $c = 0$ (the cost of lying), $B = 1$ (the number of audits), and $f(\x, \z) = x_2z_1...z_m$.
    Note that only agents with $x_2 =  1$ and $\z = 1$ are allocated a resource, and for non-constant $n$ the value of lying will always be positive.
    Under this definition of $h$, we see that given $x_1 = 0$, types are distributed uniformly. 
    However, when $x_1 = 1$ the PMF is defined conditionally on the relationship between $x_2$ and $\z$.
    The hardness of this problem arises when the principal must decide how to audit an agent reporting $\langle 1, 1, \dots, 1\rangle$. If $\Phi$ has no satisfying assignments, other than potentially $\Phi(\z) = 1$, then an agent reporting $\langle 1, 1, \dots, 1\rangle$ is guaranteed to be truthful. However,if $\Phi$ does have such an assignment, then the principal will have to audit that agent with nonzero probability. This is due to the fact that another agent, will have $x_1, x_2 = 1$, but $\z \neq 1$ and will be incentivized to lie and report $\z =1$. With out a satisfying assignment, no such incentivized type will exist.

\subsection*{Proof of Theorem~\ref{thm:bayes_nash_best_policy}}
%\begin{proof}

First note that for any realization of agents, only agents whose true type scores below the threshold, but can report a type scoring above the threshold, will have incentive to lie. Denote the set of these agent types as 
\begin{align*}
U = \{&(\x, \z)\in\inter:f(\x, \z) \geq \theta \text{ with } h(\x, \z) > 0 \text{ and } \\
&\exists \z' \text{ s. t. } f(\x, \z') < \theta \text{ with } h(\x, \z') > 0\}.
\end{align*}
 That is, $U$ is the set of all \emph{suspicious}-types.
For any set of reports $\A'$, \unf\ considers reports in $\A'$ to be in one of three categories; \emph{impossible}, \emph{suspicious}, or neither. First note that by definition, any agent regardless of their true type receives utility at most $0$ from reporting a type which falls into the ``neither" category, even when that agent is audited with probability $0$. Hence any optimal audit policy need only focus on how to audit agents whose reports fall into the other two categories, \emph{impossible} or \emph{suspicious}. 

Since the notion of optimality is defined in terms of \eBNIC, we are examining the case when all agents report their type truthfully, and one agent, say agent $i$ is considering deviating while all other agent's strategies remain fixed. As such, from the principal's perspective, there is at most one dishonest agent in any set of reports. Thus, if agents $i$ reports type $\aj_i'$ and $h(\aj_i') = 0$, the principal is immediately aware of the identity of the dishonest agent. Moreover, if some other agent $\aj_j$, considers falsely reporting some $\aj_j'$, agent $j$ knows that type $\aj_i'$ will never in appear in the set $\A'_{-j}$ and thus $\aj_j$'s utility of falsely reporting is independent of the probability with which any \emph{impossible} type is audited. Therefore auditing any \emph{impossible} type with probability $1$ is optimal.

Now we need only show that the way in which \unf\ audits \emph{suspicious} types constitutes an optimal audit policy.
Let 
\begin{align*}
    L = \{(\x, \z) \in \inter : h(\x, \z) > 0 \text{ and } \exists\z' \text{ s.t. } (\x, \z') \in U \}
\end{align*}
That is, $L$ is the set of all true types that could possibly report a \emph{suspicious} type.
Under \unf, for any realization of agents, all agents with true type in $L$ have the same expected value of lying when misreporting a type which scores above the threshold. That is, for any realization $\pazocal{A}$ and for any $\aj_i, \aj_j\in \pazocal{A}$, 
\begin{align*}
    \mathbb{E}[u_i(\aj_i', \A'_{-i})|f, \phi]& = \mathbb{E}[u_i(\aj_j', \A'_{-j})|f, \phi] \\
    &\quad\quad\forall \aj_i', \aj_j' \text{ with } f(\aj_i'), f(\aj_j') \geq \theta
\end{align*}
Let $G(\A_{-i})$ be the set of agents whose true type scores above the threshold. Then the previous equivalence can be seen by the fact that under threshold, the expected value of lying for agent $\aj_i$ when all other agents are truthful is
\begin{align*}
    &\mathbb{E}[u_i(\aj_i', \A'_{-i})|f, \phi] = \mathbb{E}_{\A'_{-i}}[1 - \phi_i(\A') - c \phi_i(\A')] \\
    =& \mathbb{E}_{\A_{-i}}[1 - \phi_i(\A_{-i} \cup\{\aj_i'\}) - c \phi_i(\A_{-i}\cup \{\aj_i'\})]\\
    & = 1 - (1 + c)\mathbb{E}_{\A_{-i}}\bigg[ \min\bigg(1, \frac{B}{|G(\A_{-i})| + 1}\bigg)\bigg]\\
     &= 1 - (1 + c)\\
     &\bigg(\sum_{\ell = B}^{n-1}\frac{B}{\ell + 1}\binom{n - 1}{\ell}\mathbb{P}_{\aj}\big(f(\aj) \geq 0\big)^{\ell}\big(1 -  \mathbb{P}_{\aj}\big(f(\aj) \geq 0\big)\big)^{n - \ell}  \\
     &+\sum_{\ell = 0}^{B - 1}\binom{n - 1}{\ell}\mathbb{P}_{\aj}\big(f(\aj) \geq 0\big)^{\ell}\big(1 -  \mathbb{P}_{\aj}\big(f(\aj) \geq 0\big)\big)^{n - \ell}\bigg).
\end{align*}
Thus the expected value of lying has no dependence on the agents particular type, or the particular type they misreport, and depends only on the fact that the agent's true type is in $L$ and their misreported type scores above the threshold.
This implies that agents $\aj_i$ and $\aj_j$ have equivalent expected values of lying.
The significance of this fact is that \unf~induces an $\varepsilon^*$BNIC where the value of $\varepsilon^*$ is tight for all agents with true type in $L$. 

We will now leverage the tightness of $\varepsilon^*$ in order to show that no other policy can achieve $\varepsilon$BNIC for $\varepsilon < \varepsilon^*$.
Let $\pazocal{A}$ again be any possible realization of agent types, which has at least one type in $L$, denote the agent of this type as $(\x_i, \z_i)$.
Then, given any audit policy $\psi$ and assuming other agents are truthful, the expected value of agent $i$ misreporting type $\aj_i'$, with $f(\aj_i') \geq 0$, is given as
\begin{align*}
    &\mathbb{E}[u_i(\aj_i', \A_{-i})|f, \psi] = 1 - (1 + c)\mathbb{E}_{\A_{-i}}[\psi_i(\A \cup \{\aj_i'\}]\\
    &= 1 - (1 + c)\\
    &\bigg(\mathbb{E}_{\A_{-i}}\big[\psi_i(\A'\big| |G(\A_{-i})| + 1 > B\big]\mathbb{P}\big(|G(\A_{-i})| + 1 > B\big)\\
    &+ \mathbb{E}_{\A_{-i}}\big[\psi_i(\A'\big| |G(\A_{-i})| + 1 \leq B\big]\mathbb{P}\big(|G(\A_{-i})| + 1 \leq B\big)\bigg)
\end{align*}
In the above term, the probability of being audited is broken into two terms conditioned on the number of agents in $G(\A_{-i})$. 
The two events, $|G(\A_{-i})| + 1 \leq B$ and $|G(\A_{-i})| + 1 > B$ represent a partition on the possible outcomes of $\A$, meaning that $\psi$ can be independently defined for events in the first term and events in the second term. 
The ability to define $\psi$ independently over these two events is of note due to the fact that when $|G(\A_{-i})| + 1 \leq B$ the principle has enough resources to audit each agent reporting above the threshold.
Thus, it is feasible to audit each agent reporting above the threshold, with probability 1, maximizes the term 
${\mathbb{E}_{\A_{-i}}\big[\psi_i(\A \cup \{\aj_i'\}\big| |G(\A_{-i})| + 1 \leq B\big]\mathbb{P}\big(|G(\A_{-i})| + 1 \leq B\big)}$.
This is identical to \unf~ when $|G(\A_{-i})| + 1 \leq B$.

It remains to be shown only that \unf~is the unique maximizer of the term 
$\mathbb{E}_{\A_{-i}}\big[\psi_i(\A \cup \{\aj_i'\}\big| |G(\A_{-i})| + 1 > B\big]$
Assuming $D$ is discrete (an identical argument works for continuous by replacing the sum with an integral), the expected value can be further dissected as 
\begin{align*}
    &\mathbb{E}_{\A_{-i}}\big[\psi_i(\A \cup \{\aj_i'\}\big| |G(\A_{-i})| + 1 > B\big] \\
    = &\sum_{A \in \binom{\inter}{n - 1}: G(A) + 1 > B}\mathbb{P}(\A_{-i} = A)\psi_i(A \cup\{ \aj_i'\}).
\end{align*}
The expected value of lying is monotonically decreasing with respect to the above term. 
To show the optimally of \unf~consider any other policy $\psi$ that differs from $\phi$. Since $\psi$ is not \unf, there must exist a set of reported types and an agent in that set for which $\psi$ and $\phi$ are different. Since $\aj_i$ was chosen arbitrarily, suppose the agent type is $\aj_i'$ and the realization is some $A_1 \cup \{\aj_i'\}$. Then we can express $\psi_i(A_1 \cup\{\aj_i'\}) = \phi_i(A_1\cup\{\aj_i'\}) + \gamma_{i, 1}$, for $\gamma_{i, 1} > 0$. Thus, there must exist some other reported type $\aj_j'\in A_1$ for which $\psi_j(A_1 \cup\{\aj_i'\}) = \phi_j(A_1\cup\{\aj_i'\}) - \gamma_{j, 1}$ for $\gamma_{j, 1} > 0$. As shown previous, the expected value of lying is tight for all agents, meaning $\varepsilon$ is strictly greater than $\varepsilon^*$ if the term $\psi_j(A_1 \cup\{\aj_i'\}) = \phi_j(A_1\cup\{\aj_i'\}) - \gamma_{j, 1}$ is not offset in the above equation, for any agent $\aj_j$ which is capable of reporting type $\aj_j'$. Therefore, there must exist some other realization $A_2$, such that $\psi_j(A_2\cup\{\aj_j'\}) = \phi_j(A_2\cup\{\aj_j'\}) + \gamma_{j, 2}$ for $\gamma_{j, 2} > 0$. Continuing this line of reasoning, there must be some other agent type in $A_2$ which has a lower audit weight under $\psi$ than $\phi$. This continues until we take weight from an agent whose audit probability has been given greater weight, i.e. an agent we have already seen before in this weight transferring process. This can be thought of as a weighted directed graph, where the nodes are agents the edges represent how much weight is shifted from one agent under a particular realization to another agent under that same realization. By the previous reasoning, this graph has no edge whose tip does not connect to the tail of another edge, i.e. all edges are part of a cycle. Assume that $\aj_i'$ and $\aj_j'$ are part of a two cycle, identical reasoning hold for any cycle length. 
We can write the terms of the expected probability of being audited, for types $\aj_i'$ and $\aj_j'$ which are affected by the weight shift as follows, first for $\aj_i'$ 
\begin{align*}
     &\mathbb{P}(\A_{-i} = A_1)\psi_i(A_1 \cup\{\aj_i'\})  + \mathbb{P}(\A_{-i} = A_2)\psi_i(A_2 \cup\{\aj_i'\})
\end{align*}
\begin{equation}\label{eq:i_EV}
    \begin{split}
     =&\mathbb{P}(\A_{-i} = A_1)\big(\phi_i(A_1\cup\{\aj_i'\}) + \gamma_{i, 1}\big) \\
     &\quad\quad\quad+ \mathbb{P}(\A_{-i} = A_2)\big(\phi_i(A_2\cup\{\aj_i'\} -\gamma_{i, 2} \big)
     \end{split}
 \end{equation}
 and for $\aj_j'$
 \begin{align*}
     &\mathbb{P}(\A_{-j} = A_3)\psi_i(A_1 \cup\{\aj_i'\})  + \mathbb{P}(\A_{-j} = A_4)\psi_i(A_2 \cup\{\aj_i'\})\\
     =&\mathbb{P}\big(\A_{-j} = (A_2\setminus\{\aj_j'\})\cup\{\aj_j'\}\big)\psi_j(A_1 \cup\{\aj_i'\})  \\
     &\quad\quad\quad+ \mathbb{P}\big(\A_{-j} = (A_2\setminus\{\aj_j'\})\cup\{\aj_j'\}\big)\psi_j(A_2 \cup\{\aj_i'\})\\
     =&\mathbb{P}\big(\A_{-j} = (A_2\setminus\{\aj_j'\})\cup\{\aj_j'\}\big)\big(\phi_j(A_1 \cup\{\aj_i'\})- \gamma_{j, 1}\big)  \\
     &+ \mathbb{P}\big(\A_{-j} = (A_2\setminus\{\aj_j'\})\cup\{\aj_j'\}\big)\big(\phi_j(A_2 \cup\{\aj_i'\})+ \gamma_{j, 2}\big)\\
     =&\mathbb{P}(\A_{-i} = A_1)\frac{h(\aj_i')}{h(\aj_j')}\big(\phi_j(A_1 \cup\{\aj_i'\})- \gamma_{j, 1}\big) \\
     &\quad\quad\quad+ \mathbb{P}(\A_{-i} = A_1)\frac{\mathbb{P}(\aj_i')}{\mathbb{P}(\aj_j')}\big(\phi_j(A_2 \cup\{\aj_i'\})+ \gamma_{j, 2}\big)
 \end{align*}
 \begin{equation}\label{eq:j_EV}
    \begin{split}
     =&\frac{h(\aj_i')}{h(\aj_j')}\bigg(\mathbb{P}(\A_{-i} = A_1)\big(\phi_j(A_1 \cup\{\aj_i'\})- \gamma_{j, 1}\big) \\
     &\quad\quad\quad+ \mathbb{P}(\A_{-i} = A_1)\big(\phi_j(A_2 \cup\{\aj_i'\})+ \gamma_{j, 2}\big)\bigg)
     \end{split}
\end{equation}
If $\varepsilon>\varepsilon^*$, then it must be the case that for $\aj_i'$ and $\aj_j'$ Equations \ref{eq:i_EV} and \ref{eq:j_EV} have greater value for some $\gamma_{i, 1}, \gamma_{i, 2} > 0$, than $\gamma_{i, 1} = \gamma_{i, 2} = 0$. Equivalently, it must be the case that 
\begin{align*}
    &\text{for $\aj_i'$: }~\mathbb{P}(\A_{-i} = A_1)\gamma_{i, 1} - \mathbb{P}(\A_{-i} = A_2)\gamma_{i, 2} > 0\\
    &\text{for $\aj_j'$: }\\
    &\quad\frac{h(\aj_i')}{h(\aj_j')}\bigg(\mathbb{P}(\A_{-i} = A_1)(-\gamma_{i, 1}) - \mathbb{P}(\A_{-i} = A_2)(-\gamma_{i, 2})\bigg) > 0\\
\end{align*}
If the first condition holds true, then $\mathbb{P}(\A_{-i} = A_1)\gamma_{i, 1} > \mathbb{P}(\A_{-i} = A_2)\gamma_{i, 2}$.
However, this would imply that the second condition is false, meaning that no policy $\psi$ an strictly decrease ${\mathbb{E}_{\A_{-i}}\big[\psi_i(\A \cup \{\aj_i'\}\big| |G(\A_{-i})| + 1 > B\big]}$ when compared to $\phi$.
Therefore, when $|G(\pazocal{A}_{-i})| + 1 > B$, the maximum expected value of lying for any agent type is achieved by $\phi$ and as shown in the other case, when $|G(\pazocal{A}_{-i})| + 1 \leq B$ auditing each agent above the threshold with probability $1$ achieves maximum expected value of lying of 0. Therefore, \unf~is the optimal audit policy in the sense that for no other policy $\psi$, the maximum expected value of lying under $\psi$ is lower than that of $\phi$.

\subsection*{Proof of Theorem~\ref{thm: unf_is_tract}}
    This result is straightforward. 
    To impalement \unf\ on any set of reports $\A'$, the principal need only determine if there exists an \impos\ type, and if no such type exists, compute the set of \sus\ reports in $\A'$. Checking if there exits and \impos\ type corresponds to checking if for each $\aj_i'\in\A'$, that $h(\aj_i') > 0$. 
    Suppose for any  \emph{known} type $\x$ we can check if there exists a $\z$ such that $h(\x, \z) > 0$ and $f(\x, \z) < \theta$ in polynomial time. 
    Then to check if a report, say $\aj_i'$, is \sus\ the principal need only check the existence of such a $\z$ for $\x_i$, and then check if $h(\aj_i') > 0$. 
    Each of these can be done in polynomial time and for any set of reports $\A'$ there are $n$ such checks that need to be done. Once the principal has checked each $\aj_i' \in \A'$, the set of \sus\ agents has been determined and thus \unf\ can be implanted in polynomial time.

\subsection*{Proof of Theorem \ref{thm:hard_audit_top_k}}
    This reduction will be from vertex cover.
    The crux of this proof comes from the fact that for sufficiently small $B$ and $c$, the gain from lying will not be tight among agents. Suppose agent $1$ draws a type $\aj_1$ which has very low probability of being in the top-$k$, but can report a type $\aj_1'$ which is almost certainly in the top-$k$. In contrast, suppose agent $2$ has slightly less than $\nicefrac{1}{2}$ chance of being in the top-$k$, but can report a type which has only slightly more than $\frac{1}{2}$ chance of being in the top-$k$.  Then, prior to auditing, the expected payoff of agent $1$ is far greater than that of agent $2$. If the principal has insufficient audit strength, i.e. small $B$ and small $c$, then the expected value of agent $1$ may be greater than agent $2$, even if agent $2$ is never audited. We will show that identifying agents similar to agent $2$, those who are \sus\ but should never be audited, is hard
    
    Given a graph $G = (V, E)$, let agents be of the form $\langle x_1, \dots, x_{|V|, z_1, z_2} \rangle$ where attributes are binary. Let $c = 1/|V|$, $n = 4$, $k = 2$, $B = 1$, and $D$ be uniform. Let
    \begin{align*}
    %f(\x, z) = \bigg(\bigwedge\limits_{(v_r, v_t) \in E}(x_r \lor x_t)\bigg)\land z_1.
    g(\x) = \bigwedge_{(v_r, v_t) \in E}(x_r \lor x_t).
    \end{align*}  
    i.e. $g$ is an indicator of $\x$ representing a vertex cover.
    Let $f(\x, \z) = g(\x) z_1 + z_2$
    
    Under this construction, agents can score values $0, 1, 2, 3$. Prior to auditing the agents with the most incentive to lie will be of the form $g(\x) =1, z_1 = 0, z_2=0$, and these agents' highest utility report will be $z_1 = z_2 = 1$. Thus any report with $g(\x) = z_1 = z_2 = 1$ should have the highest audit weight in any set of reports. 
    Thus in some set of report $\A' = \{\aj_1', \aj_2', \aj_3', \aj_4'\}$, if $\aj_1'$ and $\aj_2'$ have $g(\x) = 1, \z' = \mathbf{1}$, but $\aj_3'$ and $\aj_4'$ have $g(\x) = 0, \z' = \mathbf{1}$, the principal should never audit $\aj_3'$ and $\aj_4'$ if $\aj_1'$ and $\aj_2'$ are higher utility reports. 
    For each of these type, the \emph{minimum} type is $\z^* = \mathbf{0}$. Thus, the increase in marginal gain, prior to auditing for agents $1$ and $2$ is 
    Agents $\aj_1'$ and $\aj_2'$ have expected payoff proportional to the probability that any other agent score a 3. This probability is itself directly proportional to the number of vertex covers of $G$ since $\mathbb{P}(f(\aj) = 3) = \nicefrac{\beta}{2^{|V| + 2}}$ where $\beta$ is the number of vertex covers. 
    Thus determining the relationship between the payoffs for agent's $1, 2$ and $3, 4$ is equivalent to determining if the given graph has more than $2^{|V|}\frac{1}{(1 + c)}$ vertex covers, for any $c$.

\subsection*{Proof of Theorem~\ref{thm:unfk_opt_for_DNIC}}
    Suppose the principal's objective is to induce $\varepsilon$ dominant strategy incentive compatibility for the minimum value of $\varepsilon$. Then for any type $\aj_1$, the value of falsely reporting any other type $\aj_1'$, given any set of true types $\A_{-1}$ and reported types $\A_{-1}'$ of the other $n-1$ agents, must be at most $\varepsilon$. 
    Agent $\aj_1$ knows the scores of each of the other agents' reports. 
    As such, $\aj_1$ knows the top-$k$ scoring agents in $\A_{-i}'$, and knows if their true type $\aj_1$ or any false type $\aj_1'$ will score in the top-$k$. 
    Thus, agent $1$ has binary utility prior to auditing, either they are in the top-$k$ or they are not. 
    In this sense, similar to the threshold setting, all lies, barring auditing, have the same payoff. Thus the expected value of putting forth \emph{any} report $\aj_1'$ that is in the top-$k$ must have the same payoff after auditing. Otherwise, using a similar argument to the proof of Theorem \ref{thm:bayes_nash_best_policy}, the audit weights could be shifted from some less incentivized type, to some more incentivized type. This would always result in a strict decrease in $\varepsilon$.
    Under \unfk\ all reports in the top-$k$ have the same expected payoff since \unfk\ treats all suspicious reports in the top-$k$ as being equal, regardless of their actual score.

\subsection*{Proof of Theorem~\ref{thm:thresh_hard}}
    Hardness is shown via a reduction from \#VC, which is concerned with counting the number of vertex covers of a given graph $G = (V, E)$. 
    We first show this claim for discrete agent features, and then show that the reduction can be trivially extended to include continuous features.
    
    Let $D$ be uniform, $B = 1$ and agents be ${\aj = \langle x_1, ..., x_{|V|}, z_1\rangle}$, for $x, z\in \{0, 1\}$. Set 
    \begin{align*}
        f(\x, z) = \bigg(\bigwedge\limits_{(v_r, v_t) \in E}(x_r \lor x_t)\bigg)\land z_1.
        %f(\x, z) = \big(\bigwedge_{(v_r, v_t) \in E}(x_r \lor x_t)\big)\land z_1.
    \end{align*}
    Thus an report $\aj'$ yields $f(\aj') = 1$ if and only if the \emph{known} type $\x$ constitutes a vertex cover and $z = 1$. In both threshold and top-$k$, any agent reporting $\aj'$ with $f(\aj') = 1$ is \sus.
    
    First, suppose we are in the threshold setting with $\theta = \frac{1}{2}$.
    Let $\aj_1 = \langle 1, \dots, 1, 0\rangle$, then this agent can simply report $z = 1$ to score above the threshold, and when doing so, the expected marginal gain is
    \begin{align*}
         \varepsilon = 1 - ( 1+ c)\mathbb{E}_{\aj_2}[\phi_1(\{\aj_1', \aj_2\})]
    \end{align*}
    Auditing over the set of reports $\{\aj_1', \aj_2\}$, can be broken into two cases. The first, $f(\aj_1') = 1$ and $f(\aj_2) = 0$. 
    In this case it is optimal for the principal to audit agent $1$ with probability $1$. 
    The second case is when $f(\aj_1') = f(\aj_2) = 1$. In this case, it is optimal to audit both agents with probability $\nicefrac{1}{2}$ since both reports then have the same value of being misreports.
    Thus, the utility of agent $1$ reporting $z = 1$ is given by 
    \begin{align*}
        \varepsilon =  1 - (1 + c)\big(1 - \nicefrac{1}{2}\mathbb{P}(f(\aj_2) = 1)\big)
    \end{align*}
    Let $\beta$ be the number of vertex covers of $G$.
    Then falsely reporting $z=1$ is optimal for agent $1$ when 
    \begin{align*}
        &0 < 1 - (1 + c)\big(1 - \nicefrac{1}{2}\mathbb{P}(f(\aj_2) = 1)\big)\\
        \implies & \mathbb{P}(f(\aj_2) = 1) > \frac{1}{2}-\frac{1}{2 + 2c}\\
        \implies & \frac{\beta}{2^{|V| + 1}}  > \frac{1}{2}-\frac{1}{2 + 2c}\\
        \implies & \beta > 2^{|V|}\big( 1- \frac{1}{1 + c)})
    \end{align*}
    Thus, $\varepsilon > 0$ when $\beta > 2^{|V|}\big( 1- \frac{1}{1 + c)})$. Note that for $c = 0$ the inequality always holds, and never holds for $c = 2^{|V|}$.
    Thus, if there existed a polynomial time algorithm to determine if $\varepsilon > 0$, then it determining if $\beta > 2^{|V|}\big( 1- \frac{1}{1 + c)})$ could also be done in polynomial time. 
    If such an algorithm existed, then using binary search over $c\in \{1, \dots, 2^{|V|}\}$, the value of $\beta$, i.e. the number of vertex covers, could be found in polynomial time.
    
    Next, we show that in the top-$k$ a similar argument holds. The key difference is that the expected value of lying is slightly altered. 
    Let $k =1$. When $B = 1$, $n =2$ and $f$ is binary, auditing can be considered in 3 cases. If both agents report $f(\aj) 1$ then both should be audited with probability $\nicefrac{1}{2}$. If only one agent reports $f(\aj) = 1$, then that agent should be audited exclusively. Lastly, when both agents report $f(\aj) = 0$ both are guaranteed to be truthful, and auditing is not necessary. Assuming that ties for the resource are broken uniformly at random, the expected marginal gain of agent $1$ falsely reporting $z = 1$ is given by
    \begin{align*}
        \varepsilon = \mathbb{P}(f(\aj_2) = 1)\frac{3(1 - 2c)}{4} -\frac{1}{2}
        &= \frac{\beta}{2^{|V|}}\frac{3(1 - 2c}{4} - \frac{1}{2}
    \end{align*}
    and we can again use a similar searching technique over $c$ to find the value of $\beta$.
    
    In the case of continuous agent features, we can modify $f$ such that feature values are ``binned". For example, suppose that $D$ is uniform over $[0, 1]^{d+ s}$. Then we can define a truncation function, $g(\aj) = \langle \lfloor x_1 + 0.5\rfloor, ..., \lfloor z_s + 0.5\rfloor \rangle$.
    Then defining a new score function $f_1$ to be $f_1(a) = f(g(a))$, the problem is identical to the discrete version.

\subsection*{Proof of Theorem \ref{thm: ver_p_implies_audit_p}}
    Suppose for some $\inter$, $B$, $f$, $D$, $c$, $\theta$, and $n$, there exists a polynomial time algorithm that can compute the minimum $\varepsilon$ such that the problem instance is \eBNIC. 
    Then this algorithm can be used to construct an optimal audit policy, specifically \unf, in polynomial time. 
    To see this we can make use of Theorem \ref{thm: unf_is_tract}, which states that \unf\ is tractable if and only if for any \emph{known}-type $\x$, the corresponding \emph{minimum}-type $(\x, \z^*)$ can be determined to have scored below the threshold.
    Thus, for any set of reports $\A'$, we can determine how to audit each $(\x_i, \z_i')\in \A'$ by determining if their \emph{minimum}-type scores below the threshold.
    
    Computing this indicator can be accomplished by defining a new problem instance given by the same agent domain $\inter$ with $\hat{D} = D$, $\hat{n} = n$, and $\hat{\theta} = \theta$. 
    Further, set $\hat{B} = 1$, $\hat{c} = 0$, and $\hat{f}(\x, \z) = f(\x, \z)\mathbb{I}[\x = \x_i]$. 
    Under this score function, the only agents with possible incentive to lie will be those will \emph{known}-type $\x_i$. When auditing, the principal must consider the incentive to lie of the \emph{minimum}-type. 
    More precisely, the for a given \emph{known}-type $\x$, the agent with the most incentive to lie will be, by definition, be of the form $(\x, \z^*)$ where $\z^*$ is the \emph{minimum}-\emph{self-reported}-type with respect to the \emph{known}-type $\x$.
    Thus for any given domain of agent types, the incentive to lie is ultimately determined by the \emph{known}-type.
    In the constructed problem instance, the only agents with an incentive to lie are those with \emph{known}-type $\x_i$. Thus if $\varepsilon > 0$ for the constructed instance, then the minimum type of $\x_i$ has incentive to lie and any report $(\x_i, \z)$ with $f(\x_i, \z) \geq \theta$ should be audited. 
    
    As outlined in the proof of the optimality of \unf, one need only determine the set of agents which are to be audited for any given set of reports $\A'$, rather than over the set of all possible sets of reports. Thus, when determining which agents to audit, the principal would only need to run the verification algorithm on at most $n$ constructed instances (one for each of the unique $\x$'s in $\A'$). 
    Thus if verification could be done in polynomial time for a given instance, optimal auditing could also be done in polynomial time for that instance.

\subsection*{Proof of Theorem \ref{thm:thresh_approx_sample}}
%\begin{proof}
    For a given agent $\aj_i$, with $f(\aj_i')$, the expected value of falsely reporting some $\aj_i'$ with $f(\aj_i')$ is given by
    \begin{align*}
        u_i = 1 - \mathbb{E}[\phi_i(\A')] - c\mathbb{E}[\phi_i(\A')].
    \end{align*}
    By definition, this reported type is \emph{suspicious}.
    Under \unf\ the audit probability on agent $i$'s \emph{suspicious} report, in a given set of reports $\A'$, is $\phi_i(\A') = \min\big(1, \frac{B}{|G(\pazocal{A}')|}\}\big)$ where $G(\pazocal{A'})$ is the set of all \emph{suspicious} reports in $\A'$.
    Thus, 
    \begin{align*}
        \varepsilon^* = \big(1 - \mathbb{E}\big[\min(1 - \frac{B}{|G(\pazocal{A}')|}\big]\big) - c\mathbb{E}\big[\min(1 - \frac{B}{|G(\pazocal{A}')|}\big]
    \end{align*}
    By theorem \ref{thm:bayes_nash_best_policy}, we know that not only is \unf\ optimal, but all agents with a nonzero value of lying, have the exact same value of lying.
    Thus, the identity of the suspicious agent (agent $i$) does not matter, and so we can write $|G(\A')| = |G(\A_{-i})| + 1$
    Since $\A_{-i}$ is drawn in accordance with $D$, we can sample this set as a random variable from $D$.
    Moreover, since the \emph{minimum} type of any agent can be computed in polynomial time, we can compute $G(\A_{-i})$ in polynomial time as well. 
    This is due to the fact that any \emph{suspicious} report in $\A_{-i}$ will have a \emph{minimum} type which scores below the threshold.
    
    Thus, the audit probability on agent $i$, i.e. $\min\big(1 , \frac{B}{|G(\A_{-i}| + 1}\big)$, can be sampled by simulating the truthful type of $n - 1$ agents, in accordance with $D$, and counting the fraction of agents that spawn in $G(\pazocal{A}')$.
    
    Let $\gamma \in \Theta(1)$ and let $\bar{\phi}$ be the empirical average of $\min\big(1 , \frac{B}{|G(\pazocal{A}'|}\big)$ after $n^{\gamma}$ samples. Then, Hoeffding's inequality yields,
    \begin{align*}
        &\mathbb{P}\big(\big|\bar{\phi} - \mathbb{E}\big[ \min\big(1 , \frac{B}{|G(\pazocal{A}')|}\big)\big]\big|\leq \frac{1}{\sqrt{n^{\gamma - 1}}}\big) \\
        \geq& 1 - 2 e^{-n^{\gamma}\frac{1}{n^{\gamma - 1}}} = 1 - 2 e^{-2 n} \geq 1 - \frac{1}{n^2}
    \end{align*}
    Thus, by taking the sample average, $
    \bar{\phi}$ as an approximation of $\min\big(1 , \frac{B}{|G(\pazocal{A}'|}\big)$, we obtain
    \begin{align*}
        &|\varepsilon' - \varepsilon^*| \\
        =& \big|(1 - \mathbb{E}\big[\min\big(1 , \frac{B}{|G(\pazocal{A}')|}\big)\big] - c \mathbb{E}\big[\min\big(1 , \frac{B}{|G(\pazocal{A}')|}\big)\big]\\
        &\quad\quad\quad- (1 - \bar{\phi}) - c \bar{\phi} \big|\\
        =& (1 + c)\big|\big(\mathbb{E}\big[\min\big(1 , \frac{B}{|G(\pazocal{A}')|}\big)\big] - \bar{\phi} \big) \big|\leq (1 + c)\frac{1}{\sqrt{n^{\gamma - 1}}}
    \end{align*}
    with probability at least $1 - \frac{1}{n^{\gamma}}$.
    
     As stated previously, if $c \geq n$, the mechanism is trivially 0-BNIC.
     For $0 < c < n$ the dependency of $c$ in the run-time can be removed.
     Therefore, we have that 
     \begin{align*}
     (1 + c)\frac{1}{\sqrt{n^{\gamma - 1}}}\leq \frac{1 + \sqrt{n^2}}{\sqrt{n^{\gamma - 1}}} =  \Theta\big(\frac{1}{\sqrt{n^{\gamma - 3}}} \big)
     \end{align*}
     Thus the additive difference in the approximation of $\varepsilon^*$ is at most $\Theta\big(\frac{1}{\sqrt{n^{\gamma - 3}}} \big)$, with probability at least $1 - \frac{1}{n^2}$.

\subsection*{Proof of Corollary \ref{cor:piecewise-nashEq}}

    We first show this result for linear functions, i.e. $m = 1$.
    For linear $f$, we can write $f(\x, \z) = \w_1\x + \w_2\z$ for some weight vectors $\w_1, \w_2$. We omit the bias term for simplicity but it does not effect the analysis.
    When $f$ is of this from a report $\aj'= (\x, \z')$ is \sus\ if $f(\x, \z') = \w_1\x + \w_2\z' \geq \theta$ and there exists some $\z$ with $h(\x, \z) > 0 $ and $f(\x, \z') = \w_1\x + \w_2\z < \theta$.
    Thus, independent of $h$, we know any true type $\x$ with $\w_1\x \geq \theta - \w_2\z^*$, where $\z^* = \argmin_{\z} f(\x, \z)$ is non-\sus.
    Since the value of $\theta - \w_2\z^*$ is independent of $\x$, the set of reports which are guaranteed to be non-\sus are given by a separating hyperplane. 
    We will deal with the case of $h(\x, \z) = 0$ later.
    Let 
    \begin{align*}
        G = \{(\x, \z')\in \inter: f(\x, \z') \geq \theta \text{ and } \exists \z \text{ s.t. } f(\x, \z) < \theta\}
    \end{align*}
    Then $G$ is the set of all reports that would be \sus\ when $h > 0$.
    Using Theorem \ref{thm: tract}, the expected value of any \sus\ agent is given by
    \begin{align*}
    1 - (1+c)\sum_{\ell = 0}^{n-1}\binom{n-1}{\ell}p_U^{\ell}( 1- p_U)^{n - \ell - 1}\min\big(1, \nicefrac{B}{\ell + 1})
    \end{align*}
    where $p_U$ is the probability that any agent drawn from $D$ is $U$, the set of \sus\ types.
    Thus, all that is required is to compute $p_U$. 
    To do this, we will first compute $p_G = \mathbb{P}(\aj \in G)$ and then show that $\mathbb{\aj \in G\setminus U}$ can be computed in an equivalent way.
    Thus giving $p_U = \mathbb{P}(\aj \in G) - \mathbb{\aj \in G\setminus U}$.
    
    The value of $p_G = \int_G h(\x, \z) d\x\z$ can be computed as follows. Let $(\x^*, \z^*) = \argmax\{ f(\x, \z) : (\x, \z) \in I^d \times I^s\}$. 
    Note that $(\x^*, \z^*)$ must be in $G$. 
    Moreover, the region we need to integrate over can be defined as ${G = [a, b]^{d + s} \cap \{(\x, \z)\in \R^{d + s}:f(\x, \z)\geq 0\}}$. The set ${R = \{(\x, \z)\in \R^{s + d}: f(\x, \z) = \w^T(\x, \z) = 0\}}$ defines a separating hyperplane. For any dimension of the vector $(\x, \z)$ say $t$, and WLoG assume dimension $t$ is associated with the $x$ component of the vector. Then we know that the bounds of integration of integration over dimension $t$ will have either upper bound $b$ or lower bound $a$, since $x^*_t \in \{a, b\}$ by the monotonicity of $f$. Suppose we know the lower bound is $x^*_t = b$, then the upper bound will be either $\hat{x}_t = b$, or $\hat{x}_t\in R$. The particular value of $\hat{x}_t$ depends on the the value of the other variables. As such, we can express the bounds for the $t^{\text{th}}$ dimensions as $x^*_t = a$ and $\hat{x}_t = \min(b, \hat{b}_t)$ where $\hat{b}_t = \frac{1}{w_t}(\sum_{\ell \neq t}w_{\ell}x_{\ell} + \sum_{\ell = 1}^s w_{\ell}z{\ell})$. Symmetric definitions are given for $\hat{a}_t$ are given when the upper bound of integration is guarantied to be $b$. Therefore the bounds of integration for each dimension are given by intervals of the form $[x_t^*, \hat{x}_t] = [a, \min(b, \frac{1}{w_t}(\sum_{\ell \neq t}w_{\ell}x_{\ell} + \sum_{\ell = 1}^s w_{\ell}z_{\ell})]$ or $[\hat{x}_t, x_t^*] = [\max(a, \frac{1}{w_t}(\sum_{\ell \neq t}w_{\ell}x_{\ell} + \sum_{\ell = 1}^s w_{\ell}z_{\ell}), b]$. For each dimension the integral can be split on the min or max, yielding a linear function. This split will yield at most $d + s$ rectangular regions and one region which is defined entirely by bounds of the form $[a + \gamma_t, \frac{1}{w_t}(\sum_{\ell \neq t}w_{\ell}x_{\ell} + \sum_{\ell = 1}^s w_{\ell}z_{\ell})]$ or $[\frac{1}{w_t}(\sum_{\ell \neq t}w_{\ell}x_{\ell} + \sum_{\ell = 1}^s w_{\ell}z_{\ell}), b - \gamma_t]$ for some constant $\gamma_t$ which is given by the boundary of the rectangular regions. Therefore, the integral of $h$ over any of the $t$ dimensions is computable and $G$ is able to be broken down into $s + d + 1$ regions which each contain $s + d$ simple integrals and therefore the integral over the region $G$ is computable in polynomial time.
    Hence the maximum expected value of lying for any agent can be computed as
    \begin{align*}
        \varepsilon = 1 - &(1 + c)\sum_{\ell = 0}^{n - 1} \binom{n}{\ell + 1} \bigg(\int_G h(\x, \z)d(\x, \z)\bigg)^{\ell + 1}\\
        &\bigg(1 - \int_G h(\x, \z)d(\x,\z)\bigg)^{n - \ell - 1} \min\bigg(1, \frac{B}{\ell + 1}\bigg)
    \end{align*}
    when $h> 0$.
    However, there may be some polynomial number of intervals $[a_1, a_2]^{d + s}$ over which $h = 0$. 
    In this case, if $[a_1, a_2]^{d + s}\cap \{(\x, \z) : f(\x, \z) < \theta\}$, then the set $G$ may have non-\sus\ types and we have over counted the value of $p_U$. However, since these areas where $h =0$ are given in intervals. The sets over which we have miscounted $p_U$ are also in intervals. As such we can use the exact technique used to find $p_G$ to find $p_{G\setminus U}$ by integrating $h$ over each such interval.
    Thus we can find $p_U = p_G - p_{G \setminus U}$ for linear $f$.
    For linear $f$.
    
    To generalize this result to piece-wise linear functions we show that the above process for linear functions can be performed $m$ number of times, where $m$ is the number of piece-wise regions over which $f$ is defined.
    For each $L_t \in P$, define $f\big|_{L_s}$ as $f_s$, with the understanding that $f_s$ is only applied to elements in $L_t$.
    Determining the minimum value of $\varepsilon$ such that \unf is $\varepsilon$-BNIC is equivalent again to determining the measure of $G = \{(\x, \z) \subset I^d \times I^s: f(\x, \z) \geq 0\}$ with respect to $h$.
    The expected value of lying for any agent whose true type scores below the threshold is again 
    The value of $\int_G h(\x, \z)dG$, can again be computed by expressing the boundary conditions of $G$ as simple limits of integration.
    The key difference in the setting of piecewise linear functions is that $G$ is no longer contiguous and thus must first be broken down into contagious regions before integrating. 
    For each of the partitions $L_s\in P$ we can again have a separating hyperplane $R_s = \{ (\x, \z)\in \R^{d + s} : f(\x, \z) = \w^T(\x, \z) = 0\}$. Over each of these regions we again know that the set value $(\x^*, \z^*)_s = \argmax_{(\x, \z)\in L_s}f(\x, \z)$ is in $L_s\cap R_s$. From here, since each partition is a rectangular region. Which will gives an efficient method to compute each integral of the form $\int_{G\cap L_s}h(\x, \z)d(\x,\z)$.
    \begin{align*}
        \int_{G}h(\x, \z) d(\x, \z) = \sum_{s = 1}^{m} \int_{G\cap L_s}h(\x, \z)d(\x,\z)
    \end{align*}
    As per the linear case, we have again over counted the set of \sus\ types as $G$. But using an identical argument to the linear case, we can again construct some polynomial number of intervals which constitute the set $G\setminus U$.
    Integrating $h$ over each of these regions gives us the difference in the measure of $G$ and $U$. 
    Thus we can compute $p_U = p_G - p_{G\setminus U}$, and by Theorem \ref{thm: tract}, we have that $\varepsilon$ can be computed efficiently.

 \subsection*{Proof of Corollary \ref{thm:unf_on_PWL_top_k}}

   This proof follows a similar line of reasoning to the proof of Theorem \ref{thm: tract}.
   As discussed previously, when $\frac{(1 + c)B}{k} \geq 1$ \unf is BNIC for all agents types independent of $f$ and $D$. So assume that $\frac{(1 + c)B}{k} < 1$
   Let $T_k$ be the set of the highest $k$ scoring agents, then the expected value of an agent with true type $\aj_i$, misreporting type $\aj_i'$ under \unf~can be expressed as 
   \begin{align*}
       &\mathbb{E}_{\A_{-i}}[\alpha_i(f, \A')(1 - \phi_i(\A')) - c\phi_i(\A)' - \alpha_i(f, \A)] \\
       =& \mathbb{P}(\aj_i'\in T_k)( 1 - (1 + c)\frac{B}{k}) - \mathbb{P}(\aj_i \in T_k)
   \end{align*}
   For any reported type $\aj_i'$ the value of $\mathbb{P}(\aj_i' \in T_k)$ can treated as the CDF of a binomial random variable. For simplicity, suppose agents assume worst case tie-breaking, identical analysis holds for other simple tie breaking schemes such as random, and best case, tie breaking. If ties are broken in the worst case for agents, then an $\aj_i'$ receives the resource if there are at most $k- 1$ agents with scores at least $f(\aj_i')$. Thus $\mathbb{P}(\aj_i' \in T_k)$ is associated with a binomial random variable with $n - 1$ trials and probability of success equal to $\mathbb{P}(f(\x, \z) \geq f(\aj_i'))$. This mirrors the technique used in threshold allocation and we use an identical technique to compute those probabilities. 
  
   Once the value of $\mathbb{P}(\aj_i' \in T_k)$ and $\mathbb{P}(\aj_i \in T_k)$ are known we need only determine which agents has the highest incentive to lie. Since $f$ is linear we can write $f(\x, \z) = \w_1^T \x + \w_2^T \z$. The domain of agent types is bounded and thus there exists $\x_{\max} = \max_{\x} \w_1^T$ and $\x_{\min} = \min_{\x} \w_1^T \x$. More over there also exists $\z_{\max} = \max_{\z} \w_2^T \z$ and $\z_{\min} = \min_{\z} \w_2^T \z$.  Since $D$ is uniform the $\mathbb{P}((\x_1, \z_{\max}) \in T_k) - \mathbb{P}((\x_1, \z_{\min}) \in T_k) = \mathbb{P}((\x_2, \z_{\max}) \in T_k) - \mathbb{P}((\x_2, \z_{\min}) \in T_k)$ for any $\x_1, \x_2$. More over, since $f$ is continuous,  $\mathbb{P}((\x, \z_{\max}) \in T_k) - \mathbb{P}((\x, \z_{\min}) \in T_k)$ will take on all values in the interval 
   \begin{align*}
        &\big[\mathbb{P}((\x_{\max}, \z_{\max}) \in T_k) - \mathbb{P}((\x_{\max}, \z_{\min}) \in T_k)\\
        &\quad\quad\mathbb{P}((\x_{\min}, \z_{\max}) \in T_k) - \mathbb{P}((\x_{\min}, \z_{\min}) \in T_k)\big].
   \end{align*}
   We are interested in finding the agent type $(\x, \z_{\min})$ which has the the most incentive to lie. i.e. the largest gain for submitting $(\x, \z_{\max})$.
   We can express the value of this type as $v_1( 1 - (1 + c)\frac{B}{k}) - v_2$ Since this value is linear, and $f$ (which determines $v_1$, and $v_2$ is linear) this value is maximized at one of the extremes. Thus $v_1 = \mathbb{P}((\x_{\max}, \z_{\max}) \in T_k)$ and $v_2 = \mathbb{P}((\x_{\max}, \z_{\min}) \in T_k)$, 
   or $v_1 = \mathbb{P}((\x_{\min}, \z_{\max}) \in T_k)$ and $v_2 = \mathbb{P}((\x_{\min}, \z_{\min}) \in T_k)$.
    Each of these values are computable in polynomial time, by directly taking the ideas in the proof of Corollary \ref{cor:piecewise-nashEq} and integrating the measure of $h$ over the set $G = \{(\x, \z'): f(\x, \z') \geq \theta \text{ and } \exists\z \text{ s.t. } f(\x, \z) < \theta\}$, where $\theta\in \{f(\x_{\max}, \z_{\max}), f(\x_{\max}, \z_{\min}), f(\x_{\min}, \z_{\max}), f(\x_{\min}, \z_{\min}\}$ 
    Once $p_G$ is computed for each value. We know the probability that that each of these types scores in the top-$k$, via a binomial CDF with $n-1$ trials, and success rate $p_G$. 
    Thus we have the values of $v_1, v_2$, which give us the expected value of lying for the most incentivzed agent, i.e. $v_1( 1 - (1 + c)\frac{B}{k}) - v_2$.

%\begin{theorem}
%         Suppose the distribution of agent types is well-behaved, with PDF $h > 0$, over the domain of types, $f$ is piecewise linear, and $\alpha(f, \A')$ is top-$k$ allocation.
%        Then computing the policy \wgh~for any set of reported types $\A'$, and determining the minimum $\varepsilon \geq 0$ such that \wgh~is $\varepsilon$-BNIC, can both be done in polynomial time.
%\end{theorem}

\subsection*{Proof of Corollary \ref{thm:sigmoid}}

    This result follows directly from the proof of Corollary \ref{cor:piecewise-nashEq} and Theorem \ref{thm: tract}. 
    The key difference being that agents are now scored via a sigmoid function, rather than a linear function. 
    However, since allocation decisions are made via a threshold, i.e. $f(\x, \z) \geq \theta$, sigmoid functions are equivalent to linear functions in the following sense
    \begin{align*}
        &\theta = f(\x, \z) = \frac{1}{e^{\w^T(\x, \z)} + 1} \iff \w^T(\x, \z) = \log(\nicefrac{1}{\theta} -1)
    \end{align*}
    Thus, we can map any problem instance with a sigmoidal scoring function and threshold $\theta$, to a problem instance with a linear scoring function and threshold $\log(\nicefrac{1}{\theta} - 1)$
    Which again give the same hyper plane as in Corollary \ref{cor:piecewise-nashEq} and the proof follows identically from there.

\subsection*{Proof of Corollary \ref{thm:unf_on_log_top_k}}
This is a direct result of the proofs from Corollary \ref{thm:unf_on_PWL_top_k} and \ref{thm:sigmoid}.

\subsection*{Proof of Theorem \ref{thm:approx_error_tractable_cases}}

    As shown in several of the other proofs, the expected value of any agent is either $0$ or is given by a the term 
    \begin{align*}
       \varepsilon^* &= 1 - ( 1 + c) \sum_{\ell = 0}^{n - 1} \binom{n-1}{\ell} p_U^{\ell}(1 - p_U)^{n - \ell - 1}\min(1, \nicefrac{B}{\ell + 1})\\
       & =1 - ( 1 + c) \bigg(\sum_{\ell = 0}^{B} \binom{n-1}{\ell} p_U^{\ell}(1 - p_U)^{n - \ell - 1} \\
       &\quad\quad\quad\quad\quad\quad+\sum_{\ell = B+1}^{n - 1} \binom{n-1}{\ell} p_U^{\ell}(1 - p_U)^{n - \ell - 1}\frac{B}{\ell + 1}\bigg)\\
    \end{align*}
    If not from the multiplicative term $ \frac{B}{\ell + 1}$, the summation would constitute s a binomial sum, which would sum to $1$. 
    Using this fact, the complementary term $\sum_{\ell = B +1 }^{n -1} \binom{n-1}{\ell} p_U^{\ell}(1 - p_U)^{n - \ell - 1} \frac{\ell + 1 -B}{\ell + 1}$ can be used to simplify $\varepsilon^*$ to
    \begin{align*}
        &1 - (1 + c)\bigg(1 - \sum_{\ell = B + 1}^{n - 1} \binom{n-1}{\ell} p_U^{\ell}(1 - p_U)^{n - \ell - 1} \frac{\ell + 1 - B}{\ell + 1}\bigg)\\
        & \geq  1 - (1 + c)\bigg(1 + \frac{n - B}{n}\sum_{\ell = B + 1}^{n -1} \binom{n-1}{\ell} p_U^{\ell}(1 - p_U)^{n - \ell - 1}\bigg)
    \end{align*}
    Using the standard technique of mapping a binomial CMF to a beta CDF, by taking the derivative of a binomial CDF w.r.t. $p_U$, and then reintegrating (via integration by parts), we can rewrite this term again as 
    \begin{align*}
        1 - (1 + c)\bigg(1 + (n - B)\binom{n -2}{B -1}\int_{0}^{p_U} x^{B-1}(1 - x)^{n - B}\bigg)
    \end{align*}
    Once in this form, suppose we have a numerical error in our calculation of $p_U$, say $\pm\gamma$. 
    In the case when $\gamma$ is positive, the negative case follows symmetrically, we can write $\varepsilon'$, the approximation of $\varepsilon^*$, as
    \begin{align*}
        &1 - (1 + c)\bigg(1 + (n - B)\binom{n -2}{B -1}\bigg(\int_{0}^{p_U} x^{B-1}(1 - x)^{n - B}\\
        &\quad\quad\quad + \int_{p_U}^{p_U + \gamma} x^{B-1}(1 - x)^{n - B}\bigg)\bigg)
    \end{align*}
    Thus we can write 
    \begin{align*}
        &|\varepsilon' - \varepsilon^*|\\
        \leq& (1 + c)(n - B)\binom{n -2}{B -1}\bigg(\int_{0}^{p_U} x^{B-1}(1 - x)^{n - B}\\
        &\quad\quad\quad + \int_{p_U}^{p_U + \gamma} x^{B-1}(1 - x)^{n - B}\bigg)\\
        &\quad-(1 + c)(n - B)\binom{n -2}{B -1}\int_{0}^{p_U} x^{B-1}(1 - x)^{n - B}\\
        =& ( 1+ c)(n - B)\binom{n -2}{B -1}\int_{p_U}^{p_U + \gamma} x^{B-1}(1 - x)^{n - B}\\
        \leq&(n - B)\binom{n -1}{B -1}\int_{p_U}^{p_U + \gamma} x^{B-1}(1 - x)^{n - B}
    \end{align*}
    Where the finally inequality comes from the assumption that $B(c +1) < n$, since otherwise incentive compatibility is trivially achieved by auditing \emph{all} agents uniformly.
    
    Thus, the additive error in $\varepsilon'$, when $p_U$ has additive error $\gamma$, is no more than $(n - B)\binom{n -1}{B -1}\int_{p_U}^{p_U + \gamma} x^{B-1}(1 - x)^{n - B}$. Although this error is not given in the most compact manner, it does offer some intuition as to the relative size of the error with respect to $\gamma$. The error term is roughly the the probability that a random beta variable is between $p_U$ and $p_U + \gamma$.
